# Supplementary material for: Strong-field gravitational lensing by black holes
Source: arXiv:1909.04691 source file (2019-09-10)
Supplement: Supplementary file 1 [file AppendixF.tex]

% Appendix F
% Behaviour of Newman--Penrose quantities at conjugate points
%------------------------------------------------------------------------------------

\chapter{Behaviour of Newman--Penrose quantities at conjugate points} \label{chap:appendix_f}

In this section, we present explicit expressions for vector quantities which arise from solving the linear system of ordinary differential equations \eqref{eqn:linear_higher_order_transport} in Chapter \ref{chap:geometric_optics_kerr}. These expressions are used in the derivation of the sub-leading order solutions to the system of transport equations \eqref{eqn:ho_transport_3}--\eqref{eqn:ho_transport_8} close to a conjugate point of multiplicity one.

The eigenvector of the matrix $M_{0}$ corresponding to the eigenvalue $n = -3$ is
\begin{equation}
\mathbf{v}^{(-3)} =
\left[
%\begin{array}{c}
    e^{i \varphi} ,
    e^{- i \varphi} ,
    e^{3 i \varphi} ,
    e^{- 3 i \varphi} ,
    e^{i \varphi}  ,
    e^{- i \varphi}  ,
    - 2 \left| \chi_{0} \right| i e^{2 i \varphi} ,
    2 \left| \chi_{0} \right| i e^{- 2 i \varphi} ,
    - 2 i \left| \chi_{0} \right| ,
    2 i \left| \chi_{0} \right|
%\end{array}
\right].
\end{equation}
The eigenvectors corresponding to the eigenvalue $n = -2$ is
\begin{align}
\mathbf{v}_{1}^{(-2)} &=
\left[
%\begin{array}{c}
    i e^{i \varphi} ,
    - i  e^{- i \varphi} ,
    3 i e^{3 i \varphi} ,
    - 3 i e^{- 3 i \varphi} ,
    i e^{i \varphi}  ,
    - i e^{- i \varphi}  ,
    4 \left| \chi_{0} \right| e^{2 i \varphi}  ,
    4 \left| \chi_{0} \right| e^{- 2 i \varphi} ,
    0 ,
    0
%\end{array}
\right]
\\
\mathbf{v}_{2}^{(-2)} &=
\left[
%\begin{array}{c}
    0 ,
    0 ,
    i e^{3 i \varphi} ,
    - i e^{- 3 i \varphi} ,
    i e^{i \varphi}  ,
    - i e^{- i \varphi}  ,
    2 \left| \chi_{0} \right| e^{2 i \varphi}  ,
    0 ,
    2 \left| \chi_{0} \right| ,
    0
%\end{array}
\right]
\\
\mathbf{v}_{3}^{(-2)} &=
\left[
%\begin{array}{c}
    i e^{i \varphi} ,
    - i  e^{- i \varphi} ,
    i e^{3 i \varphi} ,
    - i e^{- 3 i \varphi} ,
    - i e^{i \varphi}  ,
    i e^{- i \varphi}  ,
    4 \left| \chi_{0} \right| e^{2 i \varphi}  ,
    0 ,
    0 ,
    - 4 \left| \chi_{0} \right|
%\end{array}
\right]
\end{align}
Clearly, these three eigenvectors are linearly independent. The particular solution to the the inhomogeneous system of equations
\begin{equation}
\left( M_{0} + 2 I \right) \mathbf{x}_{1} = - \left( \mathbf{S_{0}} + M_{1} \mathbf{x}_{0} \right),
\end{equation}
is given by the vector
\begin{equation}
\mathbf{y}_{1} =
- \frac{1}{2} \left| \tau_{0} \right|
\left[
%\begin{array}{c}
    e^{i \varphi} ,
    e^{- i \varphi} ,
    e^{3 i \varphi} ,
    e^{-3 i \varphi} ,
    e^{i \varphi} ,
    e^{-i \varphi} ,
    0 ,
    0 ,
    0 ,
    0
%\end{array}
\right].
\end{equation}
